# Supplementary material for: Accelerated Experimental Design for Pairwise Comparisons
Source: arXiv:1901.06080 source file (2019-01-18)
Supplement: Supplementary file 1 [file Appendix.tex]

\begin{comment}
\begin{algorithm}[H]
\label{alg:greedy}
\caption{Greedy Algorithm} 
\begin{algorithmic}[1]
	\State\textit{Initialize $\mathcal{S}=\emptyset$} 
	\While{$|\mathcal{S}| \leqslant K$}\State
	$\bm{e^{*}}=\underset{(i,j)\in \mathcal{C}\setminus\mathcal{S}}{\mathbf{argmax}}f(\mathcal{S}\cup \{(i,j)\})-f(\mathcal{S})$	\State $\mathcal{S}=\mathcal{S} \cup e^{*} $
	\EndWhile
	\State \Return $\mathcal{S}$
\end{algorithmic}
\end{algorithm}

\begin{algorithm}[H]
\caption{Naive Greedy}\label{alg:naive}
\begin{algorithmic}[1] 
	\State\textit{Initialize $\mathcal{S}=\emptyset$}. 
    \State\textit{Input} $\mathbf{A}, \bm{x}_{1},\bm{x}_{2},\cdots,\bm{x}_{N}\in\mathbb{R}^{d},\Omega \subseteq \mathcal{C}=\{(i,j):  i,j\in \mathcal{N}, i<j\},|\Omega|=\omega$.
    
	\While{$\mathbf{True}$}
	\State Calculate  $\bm{x}_{e}^{T}\mathbf{A}^{-1}\bm{x}_{e}$ for all $e\in \Omega\setminus\mathcal{S}$.
	\State Find $e^{*}=\underset{e\in \Omega\setminus\mathcal{S}}{\mathbf{argmax}}~~ \bm{x}_{e}^{T}\mathbf{A}^{-1}\bm{x}_{e}$.
	\State $\mathcal{S}=\mathcal{S}\cup e^{*}$.
	
	\If{$|\mathcal{S}|\geqslant K$}
    \State \textbf{break}
    \EndIf
	\State $\mathbf{A}^{-1}=\mathbf{A}^{-1}-\frac{\mathbf{A}^{-1}\bm{x}_{e^{*}}\bm{x}_{e^{*}}^{T}\mathbf{A}^{-1}}{1+\bm{x}_{e^{*}}^{T}\mathbf{A}^{-1}\bm{x}_{e^{*}}}$.
	
	\EndWhile
	\State\Return $\mathcal{S}$
\end{algorithmic}
\end{algorithm}

\begin{algorithm}[H]
\caption{Factorization Greedy}\label{alg:factorization}
\begin{algorithmic}[1] 
	\State\textit{Initialize $\mathcal{S}=\emptyset$}. 
    \State\textit{Input} $\mathbf{A}, \bm{x}_{1},\bm{x}_{2},\cdots,\bm{x}_{N}\in\mathbb{R}^{d},\Omega \subseteq \mathcal{C}=\{(i,j):  i,j\in \mathcal{N}, i<j\},|\Omega|=\omega$.
	\While{$\mathbf{True}$}
	\State Calculate $\mathbf{U}$: decompose the matrix$\mathbf{A}^{-1}$ into $\mathbf{U}^{T}\mathbf{U}$ by Cholesky decomposition.
	
	\State Calculate and save  $\bm{z}_{i}=\mathbf{U}\bm{x}_{i}$ for all $i\in \mathcal{N}$. 
	\State Calculate  $d_{e}=||\bm{z}_{e_{i}}-\bm{z}_{e_{j}}||_{2}^{2}$ for all $e\in \Omega\setminus\mathcal{S}$.
	\State Find $e^{*}=\underset{e\in \Omega\setminus\mathcal{S}}{\mathbf{argmax}}~~ d_{e}$. 
	\State $\mathcal{S}=\mathcal{S}\cup e^{*}$.
	\If{$|\mathcal{S}|\geqslant K$}
    \State \textbf{break}
    \EndIf
	\State $\mathbf{A}^{-1}=\mathbf{A}^{-1}-\frac{\mathbf{A}^{-1}\bm{x}_{e^{*}}\bm{x}_{e^{*}}^{T}\mathbf{A}^{-1}}{1+\bm{x}_{e^{*}}^{T}\mathbf{A}^{-1}\bm{x}_{e^{*}}}$.
	\EndWhile
	\State\Return $\mathcal{S}$
\end{algorithmic}
\end{algorithm}

\begin{algorithm}[H]
\caption{Memoization Greedy}\label{alg:memoization}
\begin{algorithmic}[1]
	\State\textit{Initialize $\mathcal{S}=\emptyset$}. 
    \State\textit{Input} $\mathbf{A}, \bm{x}_{1},\bm{x}_{2},\cdots,\bm{x}_{N}\in\mathbb{R}^{d},\Omega \subseteq \mathcal{C}=\{(i,j):  i,j\in \mathcal{N}, i<j\},|\Omega|=\omega$.
    \State Calculate $\mathbf{U}$: decompose the matrix$\mathbf{A}^{-1}$ into $\mathbf{U}^{T}\mathbf{U}$ by Cholesky decomposition. 
    \State Calculate and save $z_{i}=\mathbf{U}_{0}\bm{x}_{i}$ for $i\in \mathcal{N}$.
    \State Build up a dictionary for all  $d_{e}=||z_{e_{i}}-z_{e_{j}}||_{2}^{2}, e\in \Omega$.
	\While{$\mathbf{True}$}
	\State Find $e^{*}=\underset{e\in \Omega\setminus\mathcal{S}}{\mathbf{argmax}}~~ d_{e} $.
	\State $\mathcal{S}=\mathcal{S}\cup e^{*}$.
	\If{$|\mathcal{S}|\geqslant K$}
    \State \textbf{break}
    \EndIf
	\State Calculate $\bm{v}=\frac{\mathbf{A}^{-1}\bm{x}_{e^{*}}}{\sqrt{1+\bm{x}_{e^{*}}^{T}\mathbf{A}^{-1}\bm{x}_{e^{*}}}}$.
	\State Calculate and save  $z_{i}=\bm{v}^{T}\bm{x}_{i}$ for all $i\in \mathcal{N}$.
	\State $d_{e}=d_{e}-(z_{e_{i}}-z_{e_{j}})^{2}$ for all $e\in \Omega\setminus\mathcal{S}$.
	\State $\mathbf{A}^{-1}=\mathbf{A}^{-1}-\frac{\mathbf{A}^{-1}\bm{x}_{e^{*}}\bm{x}_{e^{*}}^{T}\mathbf{A}^{-1}}{1+\bm{x}_{e^{*}}^{T}\mathbf{A}^{-1}\bm{x}_{e^{*}}}$.
	
	\EndWhile
	\State\Return $\mathcal{S}$
\end{algorithmic}
\end{algorithm}

\begin{figure}[!t]
%\vskip 0.2in
\begin{center}
\centerline{\includegraphics[width=1.0\columnwidth,height=0.5\columnwidth]{pic/aucplot1.pdf}}
\caption{Average AUC for the synthetic data with feature dimension $d=20$. }
\label{fig:GM}
\end{center}
\vskip -0.2in
\end{figure}



\begin{figure}[!t]
%\vskip 0.2in
\begin{center}
\centerline{\includegraphics[width=1\columnwidth,height=0.5\columnwidth]{pic/aucplot2.pdf}}
\caption{Average AUC for the synthetic data with feature dimension $d=200$ .}
\label{fig:GM}
\end{center}
\vskip -0.2in
\end{figure}


\begin{figure}[!t]
\vskip 0.0in
\begin{center}
\centerline{\includegraphics[width=1\columnwidth]{pic/aucplotrop.pdf}}
\caption{Average AUC for ROP data as a function of $K$ with $|\mathcal{A}|=30$ initial absolute labels.}
\label{fig:RopAUC40}
\end{center}
\vskip -0.2in
\end{figure}
\begin{figure}[!t]
%\vskip 0.2in
\begin{center}
\centerline{\includegraphics[width=1\columnwidth,height=0.5\columnwidth]{pic/aucplotsushi.pdf}}
\caption{Average AUC for Sushi dataset as a function of $K$ with $|\mathcal{A}|=15$ initial absolute labels.}
\label{fig:sushi}
\end{center}
\vskip -0.2in
\end{figure}
\begin{figure}[!t]
%\vskip 0.2in
\begin{center}
\centerline{\includegraphics[width=1\columnwidth,height=0.5\columnwidth]{pic/aucplotnet.pdf}}
\caption{Average AUC for Netflix dataset as a function of $K$ with $|\mathcal{A}|=20$ initial absolute labels.}
\label{fig:sushi}
\end{center}
\vskip -0.2in
\end{figure}

\begin{algorithm}[H]
\caption{Scalar Lazy Greedy}\label{heap}
\begin{algorithmic}[1]
	\State\textit{Initialize $\mathcal{S}=\emptyset$} 
    \State\textit{Input} $\mathbf{A}\in \mathbb{S}_{+}^{d}, \bm{x}_{1},\bm{x}_{2},\cdots,\bm{x}_{N}\in\mathbb{R}^{d}, \Omega=\{(i,j):  i,j\in \mathcal{N}, i<j\}, |\Omega|=\omega.$
    
    \State Decompose matrix $\mathbf{A}^{-1}$ with the form: $\mathbf{A}^{-1}=\mathbf{U}^{T}\mathbf{U}$
    
	\State Calculate and save  $\bm{z}_{i}=\mathbf{U}\bm{x}_{i}$ for all $i\in \mathcal{N}$ 
	\State Build up  tuples for all   $(\Delta(e|\mathcal{S}_{0})=||\bm{z}_{e_{i}}-\bm{z}_{e_{j}}||_{2}^{2},0,e)$ for all $e\in \Omega$.
	\State $\mathbf{H}=[(\Delta(e_{1}|\mathbf{S}_{0}),0,e_{1}),\cdots,(\Delta(e_{\omega}|\mathbf{S}_{0}),0,e_{\omega})].$
    \State\textbf{MaxHeapify}$(\mathbf{H})$.
    \State $k=0$.
	\While{$\mathbf{True}$:}
	\State $(\_\_,\_\_,e^{*})=$heappop($\mathbf{H}$).
    \State$\mathcal{S}=\mathcal{S}\cup e^{*}$
    
    \If{$|\mathcal{S}|\geqslant K$}
    \State \textbf{break}.
    \EndIf
    
    \State Calculate $\bm{v}_{k}=\frac{\mathbf{A}^{-1}\bm{x}_{e^{*}}}{\sqrt{1+\bm{x}_{e^{*}}^{T}\mathbf{A}^{-1}\bm{x}_{e^{*}}}}$
	\State Calculate and save  $\rho_{k,i}=\bm{v}_{k}^{T}\bm{x}_{i}$ for all $i\in \mathcal{N}$.
	
	\State $k+=1$
    \State $\mathbf{A}^{-1}=\mathbf{A}^{-1}-\frac{\mathbf{A}^{-1}\bm{x}_{e^{*}}\bm{x}_{e^{*}}^{T}\mathbf{A}^{-1}}{1+\bm{x}_{e^{*}}^{T}\mathbf{A}^{-1}\bm{x}_{e^{*}}}$
    
	\State $(\Delta(e_{c}|\mathcal{S}_{t}),t,e_{c})\leftarrow \mathbf{H}[1]$.
	\While{$\mathbf{True}$:}
	\State $\Delta(e_{c}|\mathcal{S}_{k})\leftarrow \Delta(e_{c}|\mathcal{S}_{t})-\underset{t\leqslant l< k }{\sum}(\rho_{l,e_{ci}}-\rho_{l,e_{cj}})^{2}$
	\State heapreplace$(\mathbf{H}, (\Delta(e_{c}|\mathcal{S}_{k}),k,e_{c}) )$
	\State $(\Delta(e_{c}|\mathcal{S}_{t}),t,opti)\leftarrow \mathbf{H}[1]$.
	
	\If{$opti==e_{c}$}
	\State \textbf{break}.
	\Else
	\State $e_{c}=opti$
    \EndIf
\EndWhile
\EndWhile
\State\Return $\mathcal{S}$
\end{algorithmic}
\end{algorithm}
\end{comment}
